# Supplementary material for: How to Not Measure Disentanglement
Source: arXiv:1910.05587 source file (2021-03-24)
Supplement: Supplementary file 1 [file appendix.tex]

\newpage
\appendix

\section*{Supplement to ``Evaluating Disentangled Representations''}

\section{Experiments}
\label{experiments}
\subsection{Spearman rank correlation between metrics}
\label{rank_correlation}

We expand the tables given in~\citep{locatello2018challenging}, which show the correlation of Spearman ranks between different metrics, by adding \OurMeasure{}.
We show the results for two datasets: dSprites~\citep{higgins2016beta} and Cars3D~\citep{reed2015deep}, in Figure~\ref{rank_correllation}.

\begin{figure}[h]
\centering
\begin{subfigure}[t]{0.45\linewidth}
\includegraphics[clip,width=\linewidth]{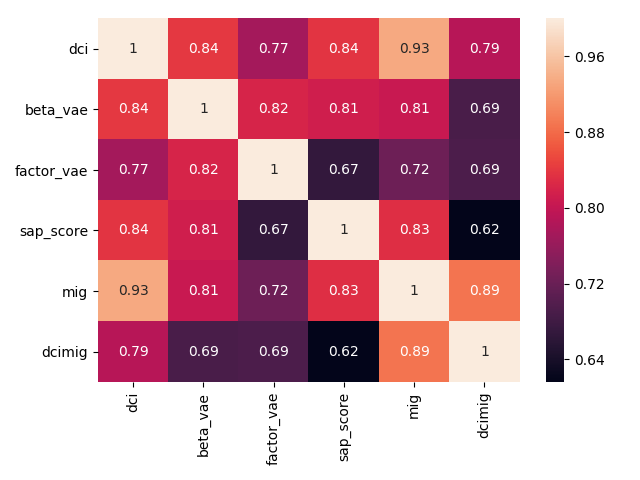}
\caption{Rank correlation of different metrics on the dSprites dataset.}
\end{subfigure}
\hfill
\begin{subfigure}[t]{0.45\linewidth}
\includegraphics[clip, width=\linewidth]{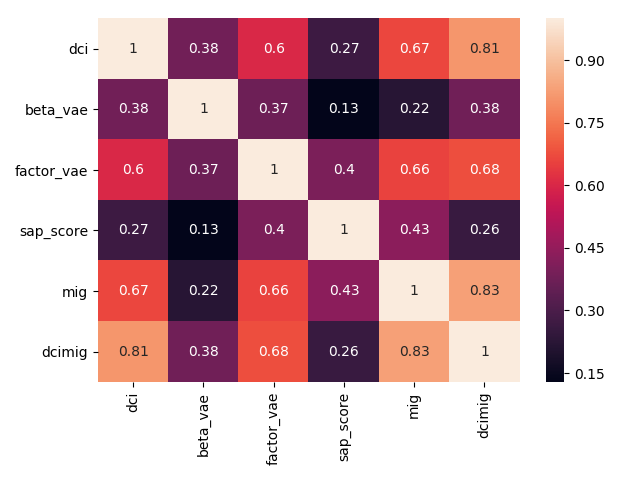}
\caption{Rank correlation of different metrics on the Cars3D dataset.}
\end{subfigure}%
\caption{Rank correlation of different metrics on two datasets. Overall, all metrics are strongly correlated.}
\label{rank_correllation}
\end{figure}

\subsection{Different behavior of  \OurMeasure{}, MIG and DCI}
\label{differences}

\subsubsection{Comparison of \OurMeasure{} and MIG}

\begin{figure}
\centering
\begin{subfigure}[t]{0.45\linewidth}
\includegraphics[clip,width=\linewidth]{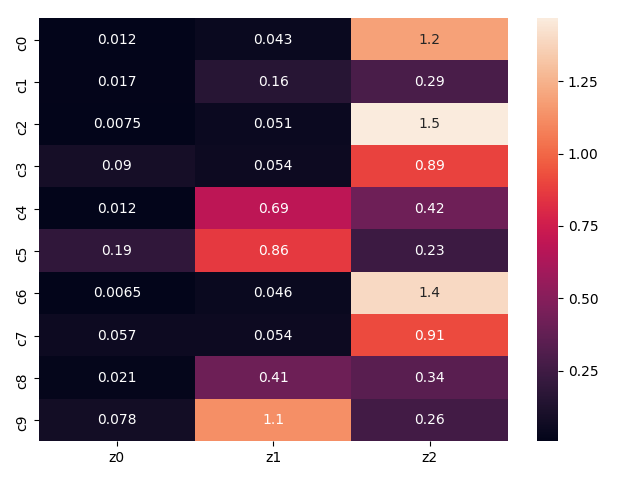}
\caption{Matrix of Informativeness, with $\mathrm{MIG}=0.05$, $\mathrm{\OurMeasure{}}=0.233$.}
\label{mig_small_dcimig_large}
\end{subfigure}
\hfill
\begin{subfigure}[t]{0.45\linewidth}
\includegraphics[clip,width=\linewidth]{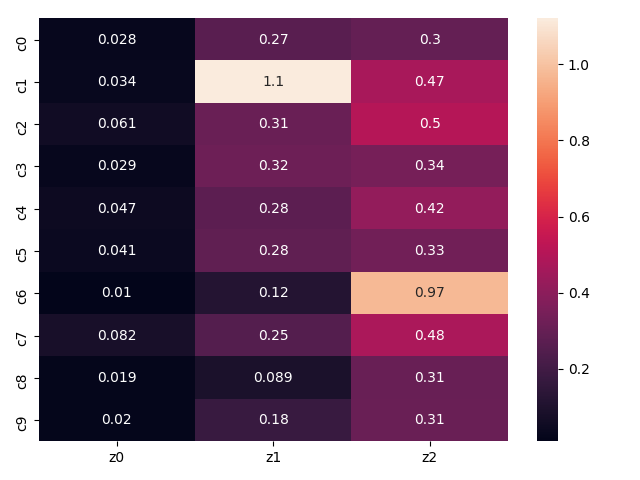}
\caption{Matrix of Informativeness, with $\mathrm{MIG}=0.12,$ $\mathrm{\OurMeasure{}}=0.15$.}
\label{mig_large_dcimig_small}
\end{subfigure}%

\label{mig_dcimig}
\caption{Matrices of informativeness of two representations, for which MIG and \OurMeasure{}, do not agree which of the two is the most disentangled one.}
\end{figure}

The representation with the matrix of informativeness given in Figure~\ref{mig_large_dcimig_small} achieves a higher MIG score than the representation with the matrix of informativeness given in Figure~\ref{mig_small_dcimig_large}.
This behavior of MIG can be explained by the fact that in the matrix of informativeness shown in Figure~\ref{mig_large_dcimig_small} only one latent factor, namely $c_1$, captures $z_1$, and only one latent factor, namely $c_6$ captures $z_2$.
On the other hand, in the matrix of informativeness shown in Figure~\ref {mig_small_dcimig_large}, there are several latent factors, namely $c_9,\ c_5$, that capture $z_1$, and also there are several hidden factors that capture $z_2$.

Now let us explain why \OurMeasure{} gives lower scores for the representation with the matrix of informativeness shown in Figure~\ref{mig_large_dcimig_small} than for a representation with the matrix of informativeness shown in Figure~\ref{mig_small_dcimig_large}.
\OurMeasure{} selects $c_1$ to reflect $z_1$ and $c_6$ to reflect $z_2$ for the representation with the matrix of informativeness shown in Figure~\ref{mig_large_dcimig_small}.
\OurMeasure{} selects $c_9$ to reflect $z_1$ and $c_2$ to reflect $z_2$ for the representation with the matrix of informativeness shown in Figure~\ref{mig_small_dcimig_large}.
But $c_1$ from Figure~\ref{mig_large_dcimig_small} is less disentangled than $c_9$ from~\ref{mig_small_dcimig_large}: $c_1$ from Figure~\ref{mig_large_dcimig_small} captures both $z_1$ and $z_2$.
In addition, $c_6$ from Figure~\ref{mig_large_dcimig_small} is less disentangled than $c_2$ from Figure~\ref{mig_small_dcimig_large}.
This explains why \OurMeasure{} selects the representation with the matrix of informativeness specified in Figure~\ref{mig_small_dcimig_large} as the more disentangled representation.

\subsubsection{Comparison of \OurMeasure{} and DCI}

\begin{figure}
\centering
\begin{subfigure}[t]{0.45\linewidth}
\includegraphics[clip,width=\linewidth]{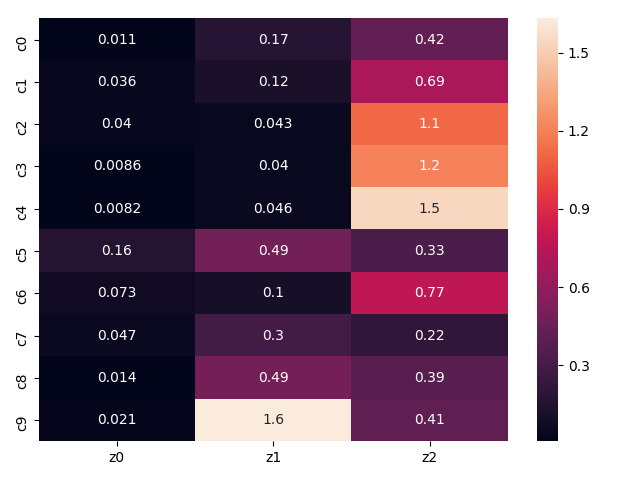}
\caption{Matrix of Informativeness, with $\mathrm{DCI}=0.38$, $\mathrm{\OurMeasure{}}=0.28$.}
\label{dci_small_dcimig_large}
\end{subfigure}
\hfill
\begin{subfigure}[t]{0.45\linewidth}
\includegraphics[clip,width=\linewidth]{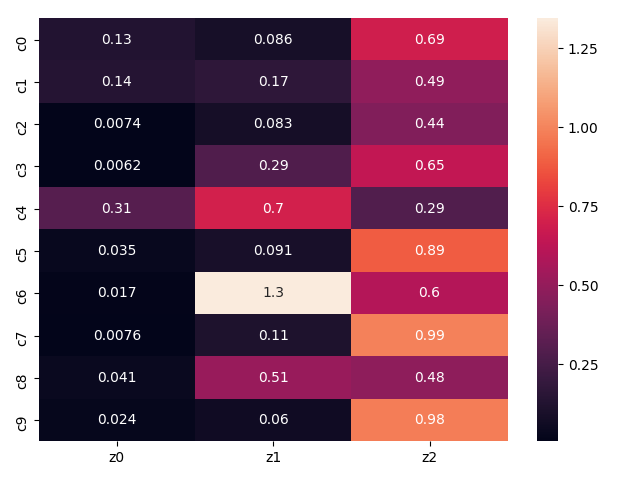}
\caption{Matrix of Informativeness, with $\mathrm{DCI}=0.42$, $\mathrm{\OurMeasure{}}=0.17$.}
\label{dci_large_dcimig_small}
\end{subfigure}%

\label{dci_dcimig}
\caption{Matrices of informativeness of two representations, for which DCI and \OurMeasure{}, do not agree which of the two is the most disentangled one.}
\end{figure}

The representation with the matrix of informativeness given in  Figure~\ref{dci_large_dcimig_small} achieves a higher DCI score than the representation with the matrix of informativeness given in Figure~\ref{dci_small_dcimig_large}.
This behavior of DCI can be explained by the fact that in the matrix of informativeness shown in Figure~\ref{dci_large_dcimig_small} there are only two entangled latent factors, namely $c_1,\ c_8$, while in Figure~\ref{dci_small_dcimig_large} four latent factors are entangled ($c_0, c_5, c_7, c_8$).
It is worth noting that in the representation with the matrix of informativeness shown in Figure~\ref{dci_large_dcimig_small}, there are many latent factors that capture the same generative factors.

Now let us explain why \OurMeasure{} gives lower scores for the representation with the matrix of informativeness shown in Figure~\ref{dci_large_dcimig_small} than for the representation with the matrix of informativeness given in Figure~\ref{dci_small_dcimig_large}.
For the representation with the matrix of informativeness given in Figure~\ref{dci_large_dcimig_small}, \OurMeasure{} selects $c_6$ to reflect $z_1$ and $c_9$ to reflect $z_2$.
For the representation with the matrix of informativeness given in  Figure~\ref{dci_small_dcimig_large}, \OurMeasure{} selects $c_9$ to reflect $z_1$ and $c_4$ to reflect $z_2$.
But $c_6$ from the Figure~\ref{dci_large_dcimig_small} is less disentangled than $c_9$ from  Figure~\ref{dci_small_dcimig_large}, $c_9$ from Figure~\ref{dci_large_dcimig_small} is less disentangled than $c_4$ from Figure~\ref{dci_small_dcimig_large}.
This explains why \OurMeasure{} selects the representation with the matrix of informativeness specified in Figure~\ref{dci_small_dcimig_large} as the more disentangled representation.
